# Supplementary material for: ADS-Edit: A Multimodal Knowledge Editing Dataset for Autonomous Driving Systems
Source: arXiv:2503.20756 source file (2025-08-05)
Supplement: Supplementary file 1 [file appendix.tex]

\appendix
\section{Metrics}

\paragraph{Reliability.}
Reliability is to evaluate the success of behavioral modification in the target driving scenarios.
% the success of change prediction from $y_o$ to $y_e$.
Intuitively, what we need is an updated $\theta_e$ with $f(t_e, m_e; \theta_e)=y_e$. 
To measure the reliability, we use the editing accuracy, as follows:
\begin{equation}
\mathcal{M}_{rel} = \mathbb{E}_{(t_e, m_e, y_e) \sim \mathcal{D}_{\text{e}}} \{ f \left( t_e, m_e; \theta_e \right) = y_e \}
\end{equation}
where $\theta_e$ refers to the parameters after editing.

\paragraph{Generality.} Given similar autonomous driving scenarios, generality assesses whether the edited model $f_{\theta_e}$ updates relevant knowledge within $(t_e, m_e)$ to retain the capacity for generalization, so that predict congruent outputs for equivalent inputs (e.g., rephrased textual quries, or similar autonomous driving's videos).
We evaluate text generality and multimodal generality as follows:
\begin{equation}
\mathcal{M}^{text}_{gen} = \mathbb{E}_{t_r \sim \mathcal{N}(t_e)} \{ f \left( t_r, m_e; \theta_e \right) = y_e \}
\end{equation}
\begin{equation}
\mathcal{M}^{mm}_{gen} = \mathbb{E}_{m_r \sim \mathcal{N}(m_e) }\{ f \left( t_e, m_r; \theta_e \right) = y_e \}
\end{equation}
where $m_r$ presents the rephrased autonomous driving's image or videos, $t_r$ refers to
the rephrased textual queries, and $\mathcal{N}(x)$ denotes to in-scope objects of $x$.

\paragraph{Locality.}
After updating the model with domain-specific knowledge in autonomous driving, locality is used to evaluate whether knowledge editing preserves the model's behavior on unrelated knowledge (e.g., unimodal factual knowledge and multimodal commonsense knowledge).
Following \citep{cheng2023mmedit}, we employ both text locality and multimodal locality to assess the stability of the editing process:
\begin{equation}
\mathcal{M}^{text}_{loc} = \mathbb{E}_{(t, Y) \sim \mathcal{D}_{\text{loc}} } \{f \left( t; \theta_e\right) = f\left(t; \theta \right)\}
\end{equation}
\begin{equation}
\begin{split}
\mathcal{M}^{mm}_{loc} = \mathbb{E}_{(t, m, y) \sim \mathcal{D}_{\text{loc-v}} } \{f \left(t, m; \theta_e\right) = f\left(m, t; \theta \right)\}
\end{split}
\end{equation}
where $\mathcal{D}_{\text{loc}}$ and $\mathcal{D}_{\text{loc-v}}$ are distinct from $\mathcal{D}_{\text{e}}$. The tuples $(t, y)$ and $(t, m, y)$ represent samples drawn from $\mathcal{D}_{\text{loc}}$ and $\mathcal{D}_{\text{loc-v}}$, respectively.

\section{Baselines} 
\label{appdix:baseline}
\paragraph{Prompt.}
Directly alter the model's behavior temporarily through prompts.
\paragraph{AdaLora.}
LoRA introduces low-rank matrices into Transformer layers, fine-tuning only a small subset of parameters while keeping the majority of the model frozen. Building on LoRA, AdaLoRA \citep{adalora} improves LoRA by adaptively allocating the parameter budget based on the importance of weight matrices, using SVD to prune unimportant updates. In our work, we employ AdaLoRA as the baseline for efficient knowledge editing.
\paragraph{GRACE.} GRACE \citep{grace} introduces a discrete key-value codebook approach, where edits are cached as latent space mappings without altering the original model weights. This method enables thousands of sequential edits by storing corrections in a retrieval-based codebook, ensuring minimal interference with unrelated inputs and strong locality . However, GRACE’s reliance on non-parametric representations limits its ability to generalize beyond memorized edits, as it struggles to integrate new knowledge into the model’s reasoning process.

\paragraph{WISE.}
WISE \citep{wise} uses a dual-memory architecture comprising a main memory for pretrained knowledge and a side memory for editing. A routing mechanism decides which memory to use during inference. Additionally, knowledge is partitioned into multiple subspaces through sharding to facilitate conflict-free edits, with subsequent merging of the shards into a unified side memory.

% \section{Detailed Experimental Settings}
% \label{appdix:exp}

% % \paragraph{Experimental Hypothesis}

% \paragraph{Hyperparameter Settings}

\section{Lifelong Editing Results}
\label{lifelong}
% 折线图
In real-world autonomous driving scenarios, sequential knowledge updates are often required. 
We sequentially test the effects of lifelong editing 1, 250, 500, 750, and 1000 times across four baseline methods: Prompt, AdaLora, GRACE, and WISE.
The lifelong editing results of Qwen2-VL and LLaVA-Onevision are shown in Figure~\ref{fig:seq_qwen} and Figure~\ref{fig:seq_llava}, respectively.

Regarding Reliability and Generality metrics, the performance of the four baselines shows a gradual decline, albeit with some fluctuations. 
WISE, as a memory-augmented approach, effectively alleviates the knowledge forgetting phenomenon observed in AdaLora, which relies on parameter updates.
Although the Prompt method demonstrates also effective lifelong editing performance at 250 and 500 times updates, it leds to an Out-of-Memory (OOM) error after 750 times updates.
% Notably, the Prompt merges multiple data updates and then input LMMs, which led to an Out-of-Memory (OOM) error after 750 times updates.
Due to the long tokens of multimodal inputs, the codebook struggles to differentiate between distinct representation information, resulting in suboptimal lifelong editing performance for GRACE.

Methods that preserve the original parameters, such as WISE and GRACE, achieved 100\% performance on the Locality metric.
Due to interference from additional inputs, the Prompt method performs poorly on the Locality metric, with even worse results observed in multimodal locality.
AdaLoRA employs low-rank matrix-based parameter updates, which minimally affect the original parameters, resulting in a strong performance on the locality metric.

\section{Benchmark Construction Details}
\label{appdix:bench}
The prompt templates are as shown in Table~\ref{tab:simplify}, Table~\ref{tab:question}, Table~\ref{tab:qa-general} and Table~\ref{tab:qa-driving}.

\section{Case of \ds benchmark}

The case of \ds benchmark is as shown in Figure~\ref{fig:video_case}, Figure~\ref{fig:multi_case} and Figure~\ref{fig:single_case}

\newpage
\begin{figure*}[h] 
\centering
\includegraphics[width=0.95\textwidth]{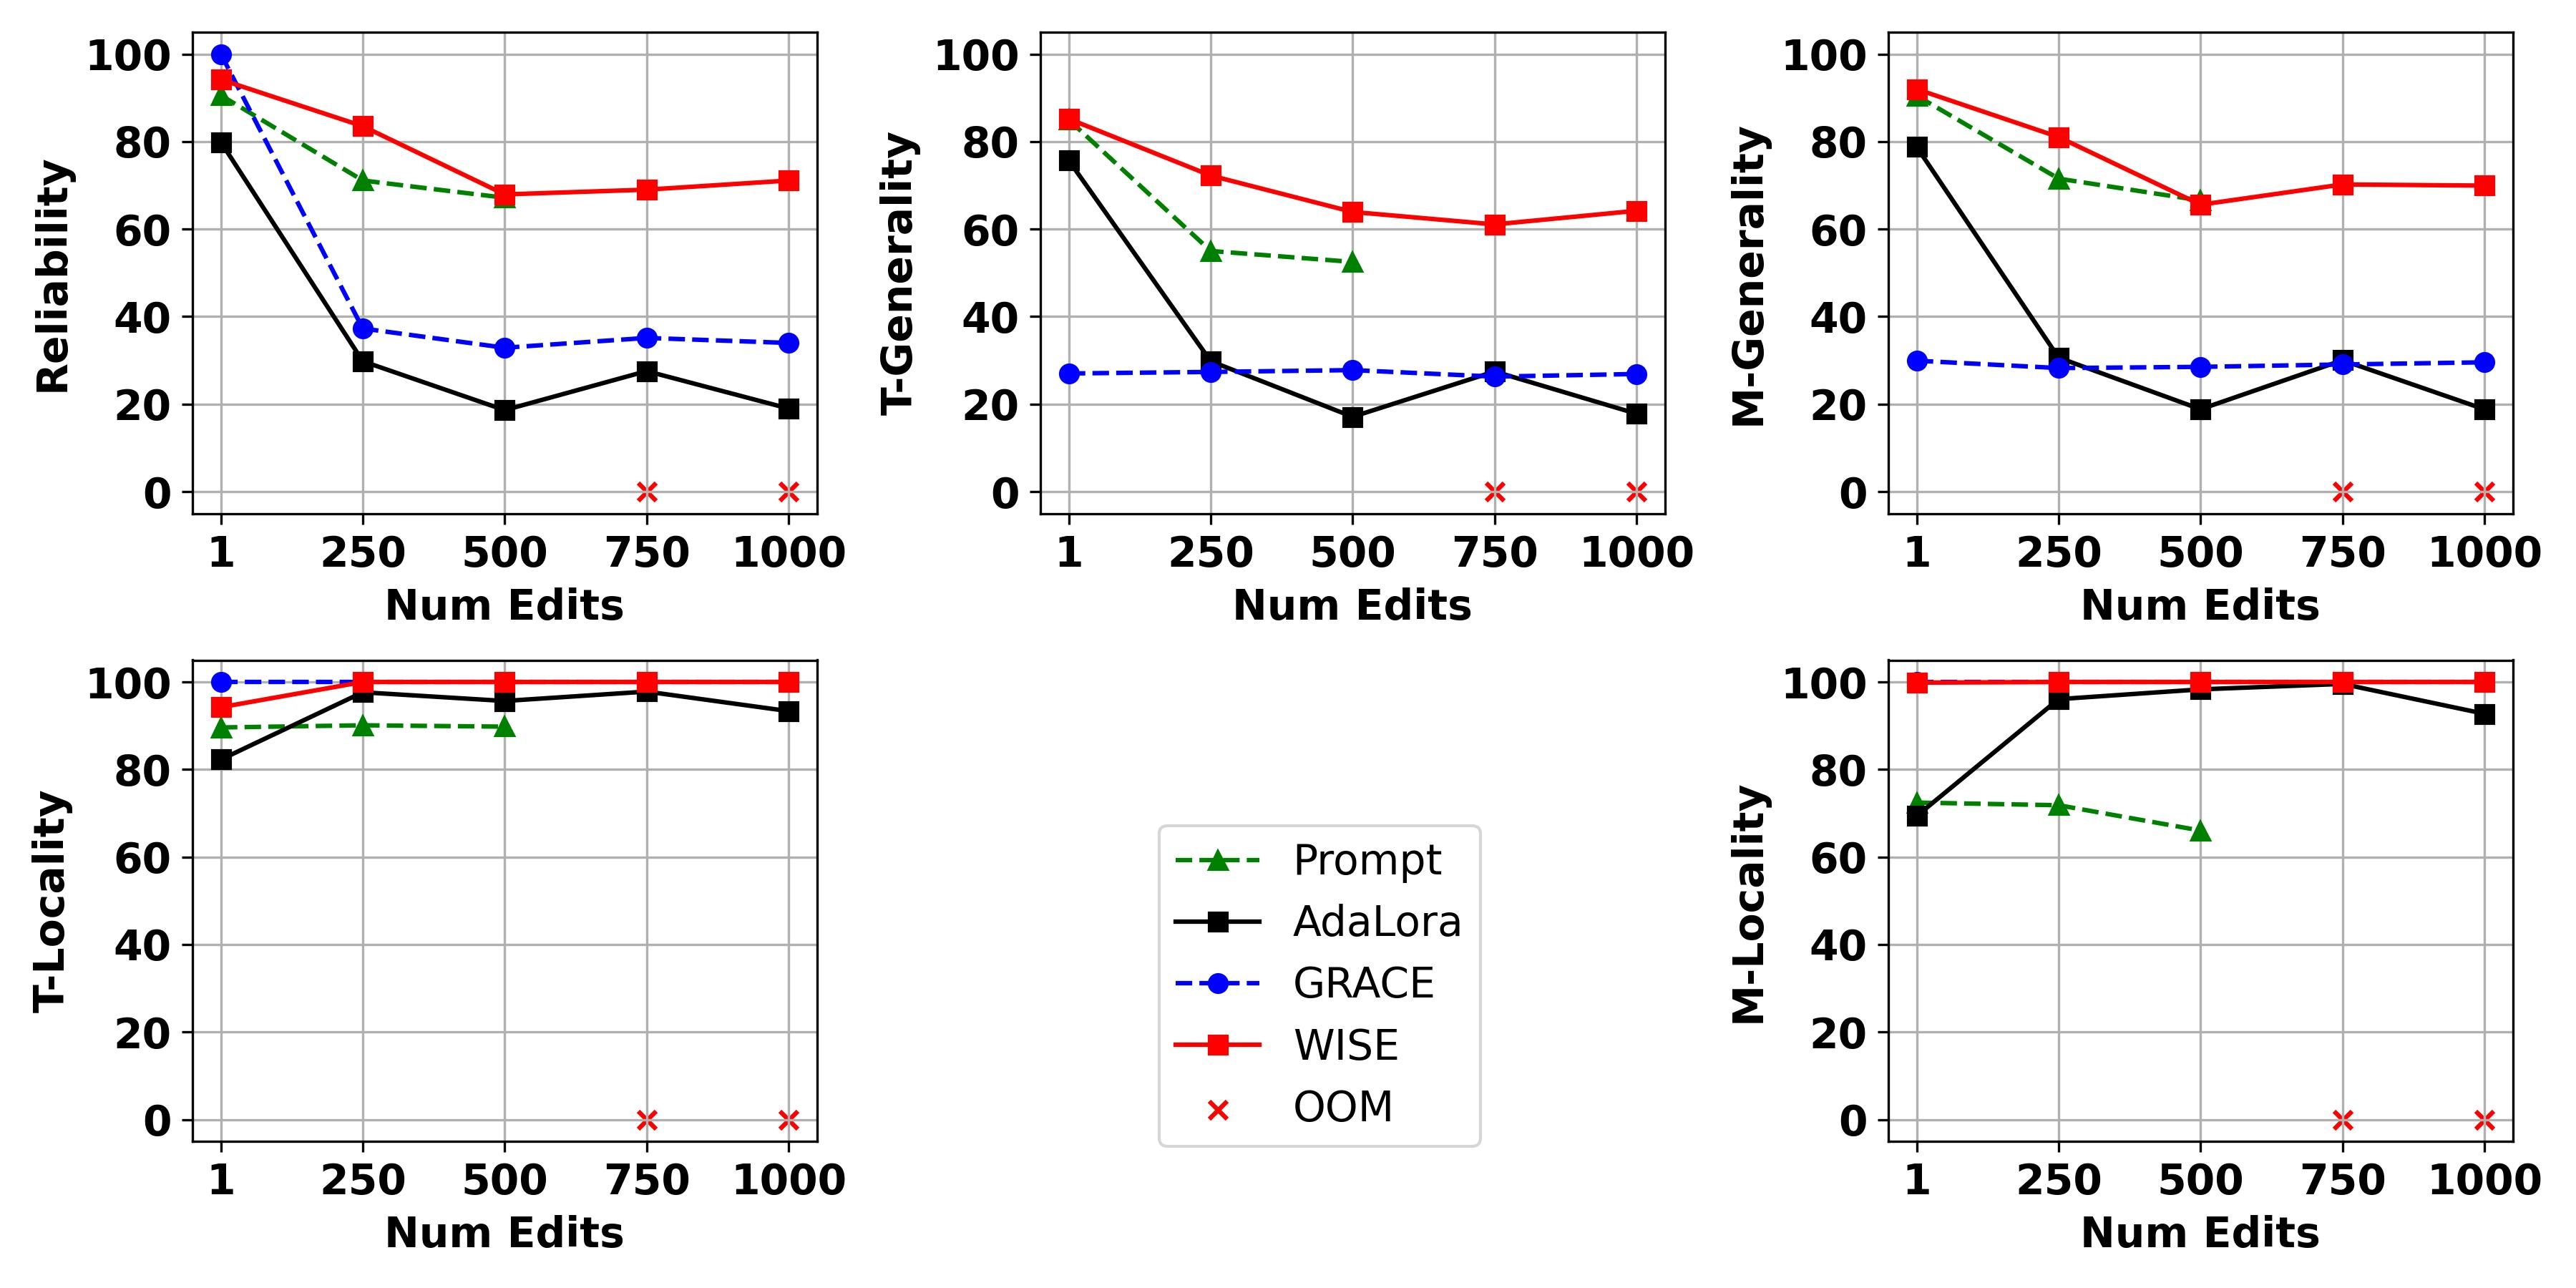}
\caption{Lifelong Editing results of Qwen2-VL. \textcolor{red}{\texttimes} indicates that Prompt triggers an Out-of-Memory (OOM) error at 750 and 1000 editing iterations.}
\label{fig:seq_qwen} 
\end{figure*}

\begin{figure*}[h] 
\centering
\includegraphics[width=1\textwidth]{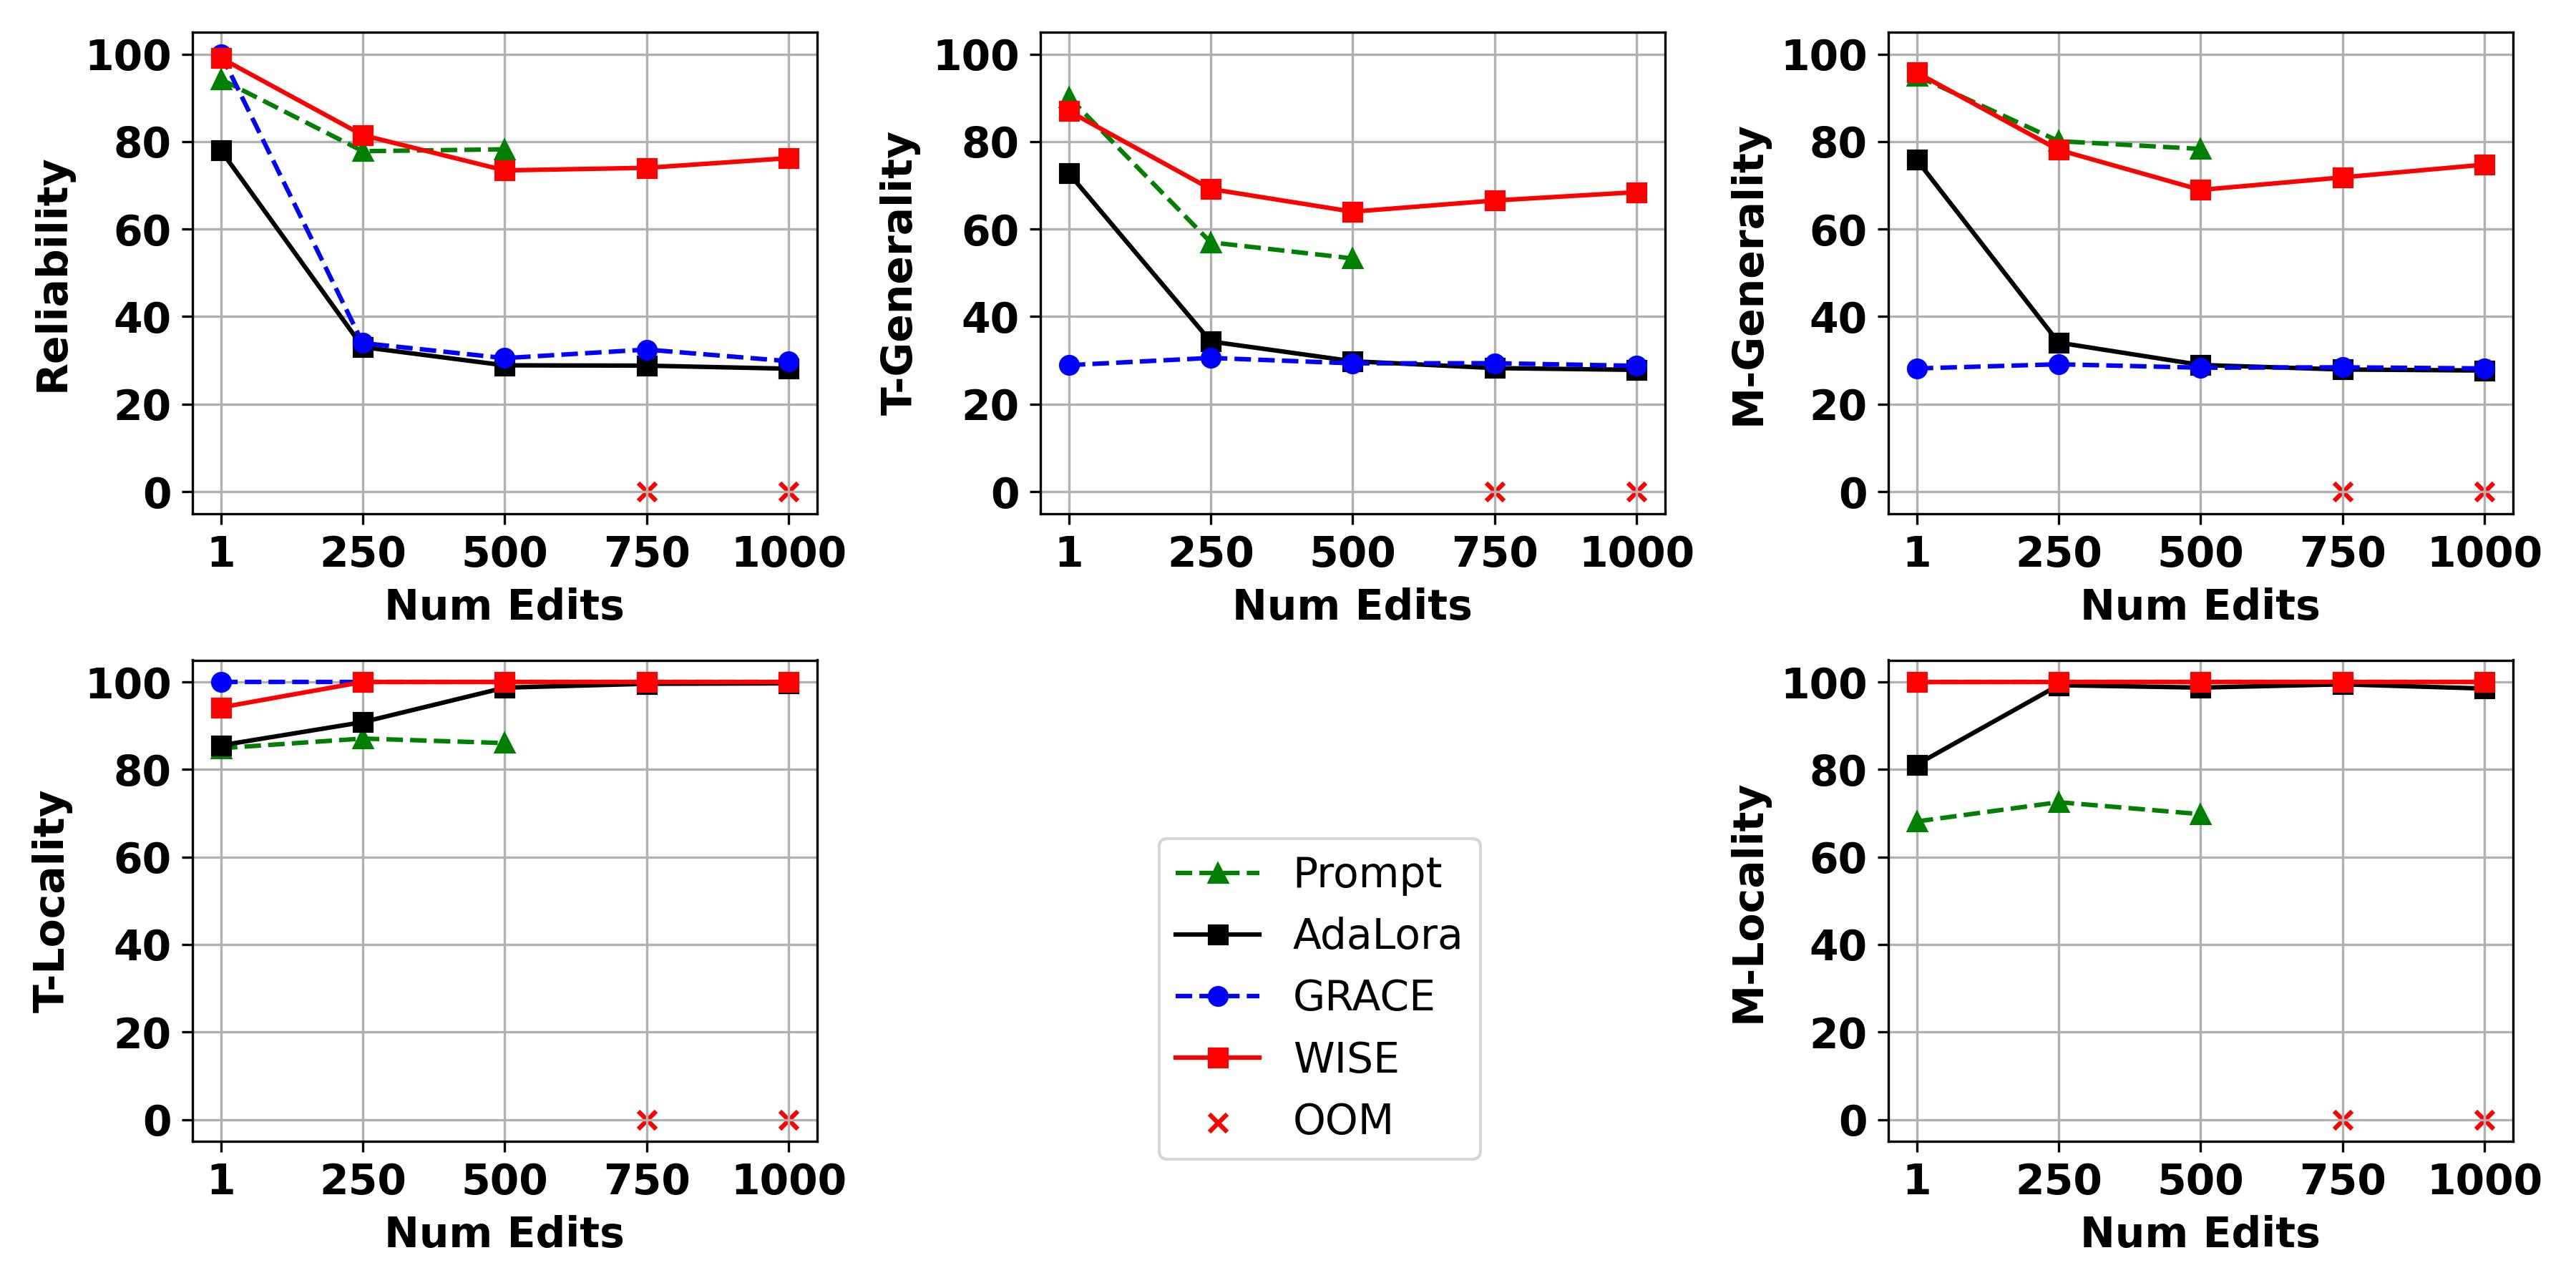}
\caption{Lifelong Editing results of LLaVA-OneVision. \textcolor{red}{\texttimes} indicates that Prompt triggers an Out-of-Memory (OOM) error at 750 and 1000 editing iterations.}
\label{fig:seq_llava} 
\end{figure*}

\begin{table*}[h]\centering
\begin{minipage}{0.85\textwidth}
%\vspace{0mm}    
\centering
\begin{tcolorbox} 
    \centering
   
     %\hspace{-4mm}
      \small
    \begin{tabular}{p{0.95\textwidth}}
   \textcolor[rgb]{0.8,0.3,0}{ {\bf SYSTEM:} } \\ 
    You are a helpful assistant. \\ \\
  \textcolor[rgb]{0.8,0.3,0}{ {\bf USER:} } \\ 
    Given a question and an answer in the VQA task, you are required to condense the answer into 1 to 5 words. You MUST FOLLOW THE FOLLOWING RULES: \\
    1. The condensed answer must be fewer than 5 tokens. \\
    2. The condensed answer must retain the core meaning of the original answer. \\
    3. Return only the condensed answer. DON'T RESPOND ANYTHING ELSE! \\ \\
    Here are some examples:\\
    <example 1>\\
    question: What is the current action and its justification? Answer in the form "action, justification".\\
    original answer: The car starts and moves right, because the vehicle in front is pulling away at the green traffic light and then it needs to go around the construction sign on the left of the road.\\
    condensed answer: Moves right.\\ \\
    <example 2> \\
    question: Is there a traffic light? If yes, what color is displayed? \\
    original answer: Yes, a temporary traffic light. It is showing green. \\
    condensed answer: Yes, green. \\
    \\
    <example 3> \\
    question: How many pedestrians are present in this image? \\
    original answer: There are no relevant pedestrians, but there is one on the left side-road and one on the right side of the road. \\
    condensed answer: No pedestrians. \\
    \\
    question: \{question\} \\
    original answer: \{answer\} \\
    condensed answer: 
    \\
    \end{tabular}
\end{tcolorbox}
%\vspace{-2mm}
\caption{Prompt template of answers simplification.}
\label{tab:simplify}
\end{minipage}
\end{table*}

\begin{table*}[h]\centering
\begin{minipage}{0.85\textwidth}
%\vspace{0mm}    
\centering
\begin{tcolorbox} 
    \centering
   
     %\hspace{-4mm}
      \small
    \begin{tabular}{p{0.95\textwidth}}
   \textcolor[rgb]{0.8,0.3,0}{ {\bf SYSTEM:} } \\ 
    You are a helpful assistant. \\ \\
  \textcolor[rgb]{0.8,0.3,0}{ {\bf USER:} } \\ 
   Given a question in the Automatic Driving QA task, you are required to rewrite the question in a different way. 
You MUST FOLLOW THE FOLLOWING RULES: \\
    1. The rephrased question should not have a high degree of overlap with the original wording. \\
    2. The rephrased question should be consistent with the core meaning of the original question. \\
    3. Return only the rephrased question. DON'T RESPOND ANYTHING ELSE! \\ \\
    
    Here are some examples: \\
    <example 1> \\
    original question: What is the current action and its justification? Answer in the form \"action, justification\". \\
    rephrased question: What is the action being performed at the moment, and what is the reasoning behind it? Please respond with "action, reasoning." \\ \\
    
    <example 2> \\
    original question: How many pedestrians are in the video? \\
    rephrased question: What is the number of pedestrians depicted in the video? \\ \\
    
    <example 3> \\
    original question: Is there a traffic light? If yes, what color is displayed? \\
    rephrased question: Does a traffic light exist, and if so, what is its current color? \\ \\
    
    original question: \{question\} \\
    rephrased question:

    \end{tabular}
\end{tcolorbox}
%\vspace{-2mm}
\caption{Prompt template of question rephrase.}
\label{tab:question}
\end{minipage}
\end{table*}

\begin{table*}[!ht]\centering
\begin{minipage}{0.85\textwidth}
%\vspace{0mm}    
\centering
\begin{tcolorbox} 
    \centering
     %\hspace{-4mm}
      \small
    \begin{tabular}{p{0.95\textwidth}}
   \textcolor[rgb]{0.8,0.3,0}{ {\bf SYSTEM:} } \\ 
    You are a helpful assistant. \\ \\
  \textcolor[rgb]{0.8,0.3,0}{ {\bf USER:} } \\ 
    Given a description about a road street view in Automatic Driving task, you are required to generate questions and provide corresponding answers from the description. \\
    You MUST FOLLOW THE FOLLOWING RULES: \\
    1. The questions must be related to driving from multiple perspectives, such as traffic object recognition, traffic condition analysis, and so on. \\
    2. The questions cannot be repeated. \\
    3. The corresponding answer must be condensed, such as fewer than 5 tokens. \\
    4. The content of the questions and answers must not include anything not covered in the description. \\
    5. Return only a series of Q\&A pairs in the form of a dictionary list. DON'T RESPOND ANYTHING ELSE! \\ \\
    Here are some examples: \\
    <example 1> \\
    description: In the traffic scene observed, there is one vehicle parked on the side of the road. Although it is partially obscured by darkness, it serves as an indication of a potentially active parking area where the ego car should remain vigilant for other vehicles that might enter or exit parking spots. Additionally, there is a traffic sign situated on the right that informs drivers of an upcoming pedestrian crossing. This suggests that the ego car should decrease its speed and be ready to yield to pedestrians who might be in the vicinity. \\
    Q\&A: [\{"question": "What should the ego car remain vigilant for?","answer": "Other vehicles entering/exiting"\},\{"question": "Where is the traffic sign located?","answer": "On the right"\},\{"question": "What does the traffic sign indicate?","answer": "Upcoming pedestrian crossing"\},\{"question": "What should the ego car do near the pedestrian crossing?","answer": "Decrease speed and yield"\}] \\

    <example 2> \\
    description: In the traffic image, there is a small black dog on the left side of the road ahead, appearing to cross from left to right. The dog's presence and potential for unpredictable movement pose a hazard, as animals can change direction suddenly, which could lead to an accident if the autonomous vehicle does not respond correctly. There are no vehicles, traffic signs, traffic lights, traffic cones, barriers, or other objects present in the image that affect driving behavior. \\
    Q\&A: [\{"question": "Are there any vehicles on the road?","answer": "No"\},\{"question": "Are there any traffic signs present?","answer": "No"\},\{"question": "Are there any barriers on the road?","answer": "No"\}]\\
    \\
    <example 3> \\
    description: The traffic scene contains a large cement mixer truck ahead on the road, taking up most of the driving lane. The truck is equipped with rear safety features like warning lights. This vehicle significantly impacts the driving behavior of the ego car, as its size and positioning affect the car's ability to safely overtake and necessitate maintaining a sufficient following distance. Additionally, there are construction barriers and debris on the side of the road to the right. These obstructions narrow the available road space, posing potential hazards that require the ego car to drive cautiously to avoid a collision. There are no vulnerable road users, traffic signs, traffic lights, traffic cones, or other objects present in this image that affect driving conditions. \\
    Q\&A: [\{"question": "What vehicle is ahead on the road?","answer": "Cement mixer truck"\},\{"question": "What safety features does the truck have?","answer": "Warning lights" \},\{"question": "How does the truck affect the ego car?","answer": "Impacts overtaking and following distance"\},\{"question": "What is on the right side of the road?","answer": "Construction barriers and debris"\},\{"question": "How do the obstructions on the right affect driving?","answer": "Narrow the road space"\},\{"question": "Are there any vulnerable road users present?","answer": "No" \},\{"question": "Are there any traffic signs or lights in the scene?","answer": "No"\}] \\
    \\
    description: \{description\} \\
    Q\&A: \\

    \end{tabular}
\end{tcolorbox}
%\vspace{-2mm}
\caption{Prompt template of general QA pairs self-generate.}
\label{tab:qa-general}
\end{minipage}
\end{table*}

\begin{table*}[!ht]\centering
\begin{minipage}{0.85\textwidth}
%\vspace{0mm}    
\centering
\begin{tcolorbox} 
    \centering
     %\hspace{-4mm}
      \small
    \begin{tabular}{p{0.95\textwidth}}
   \textcolor[rgb]{0.8,0.3,0}{ {\bf SYSTEM:} } \\ 
    You are a helpful assistant. \\ \\
  \textcolor[rgb]{0.8,0.3,0}{ {\bf USER:} } \\ 
    Given a driving suggestion about a road street view in Automatic Driving task, you are required to generate questions and provide corresponding answers from the description. \\
    You MUST FOLLOW THE FOLLOWING RULES: \\
    1. The questions must be related to driving from multiple perspectives, such as driving suggestion, traffic condition analysis, and so on. \\
    2. The questions cannot be repeated. \\
    3. The corresponding answer must be condensed, such as fewer than 5 tokens. \\
    4. The content of the questions and answers must not include anything not covered in the description. \\
    5. Return only a series of Q\&A pairs in the form of a dictionary list. DON'T RESPOND ANYTHING ELSE! \\
    \\
    Here are some examples: \\
    <example 1> \\
    suggestion: The ego car should reduce speed and prepare to stop if necessary, giving ample space for the dog to cross safely. Maintain vigilant observation of the dog's movements and be prepared for sudden changes in its direction. Furthermore, due to the narrowness and environment of the road, the ego car should drive cautiously, being alert for other potential obstacles or road users that may emerge from the side buildings or alleys. \\
    Q\&A: [\{"question": "What should the ego car do regarding speed?","answer": "Reduce speed"\},\{"question": "Why should the ego car drive cautiously?","answer": "Narrow road and potential obstacles"\},\{"question": "What other hazards should the driver be alert to?","answer": "Side buildings or alleys"\}] \\
    \\
    <example 2> \\
    suggestion: Given the proximity to the heavy vehicle ahead and the construction debris to the side, the ego car should maintain a safe following distance, prepare to slow down or stop if the mixer truck's behavior indicates impending stops or turns and refrain from attempting to overtake unless the opposite lane is visibly clear and safe to do so. The ego car should also be prepared for potential hazards from the construction area, such as entering construction vehicles or workers, and remain vigilant for any changes in road width or conditions. \\
    Q\&A: [\{"question": "What distance should the ego car maintain?","answer": "Safe following distance"\},\{"question": "What hazards should the driver be prepared for?","answer": "Construction vehicles or workers"\}] \\
    \\
    <example 3> \\
    suggestion: Given the wet road conditions, it is recommended that the ego car reduces its speed to ensure a safe stopping distance from the vehicle ahead. It should monitor the green traffic light for changes and be prepared to stop if it switches to yellow or red. The ego car should remain in the current lane, as the presence of vehicles in the left lane may hinder safe lane changing, and the road ahead seems to be leading to an exit which is partially blocked by barriers, making it inaccessible. Adherence to the road signage for navigation should be maintained, but no immediate action is required since there is no indication of an upcoming turn or exit that is accessible. Always be observant for any road users that might appear unexpectedly. \\
    Q\&A: [\{"question": "What should the ego car do due to wet road conditions?","answer": "Reduce speed"\},\{"question": "Which lane should the ego car stay in?","answer": "Current lane"\},\{"question": "Why should the ego car avoid changing lanes?","answer": "Left lane vehicles may hinder"\}] \\
    \\
    suggestion: \{suggestion\} \\
    Q\&A: \\
    \end{tabular}
\end{tcolorbox}
%\vspace{-2mm}
\caption{Prompt template of driving suggestion QA pairs self-generate.}
\label{tab:qa-driving}
\end{minipage}
\end{table*}

\begin{figure*}[ht] 
\centering
\includegraphics[width=0.6\textwidth]{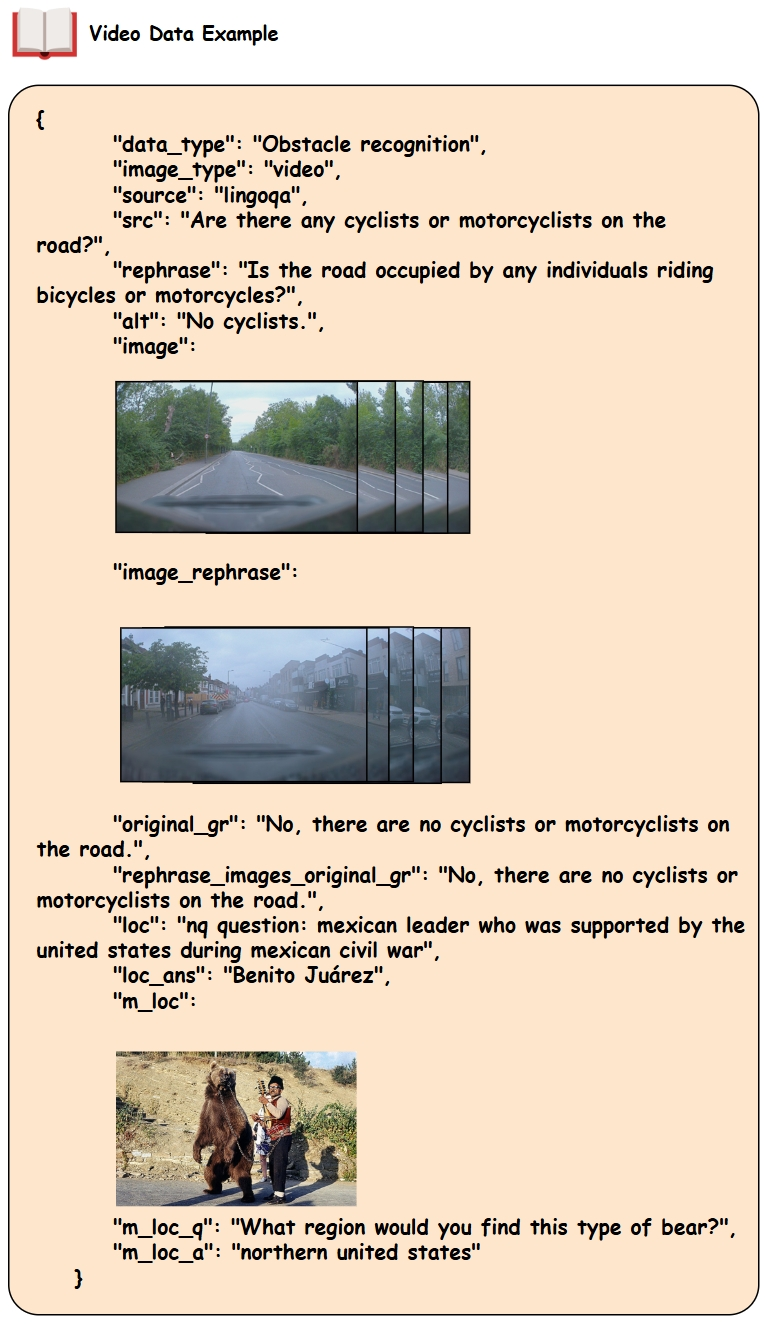}
\caption{A video data case of \ds benchmark.}
\label{fig:video_case} 
\end{figure*}

\begin{figure*}[ht] 
\centering
\includegraphics[width=0.6\textwidth]{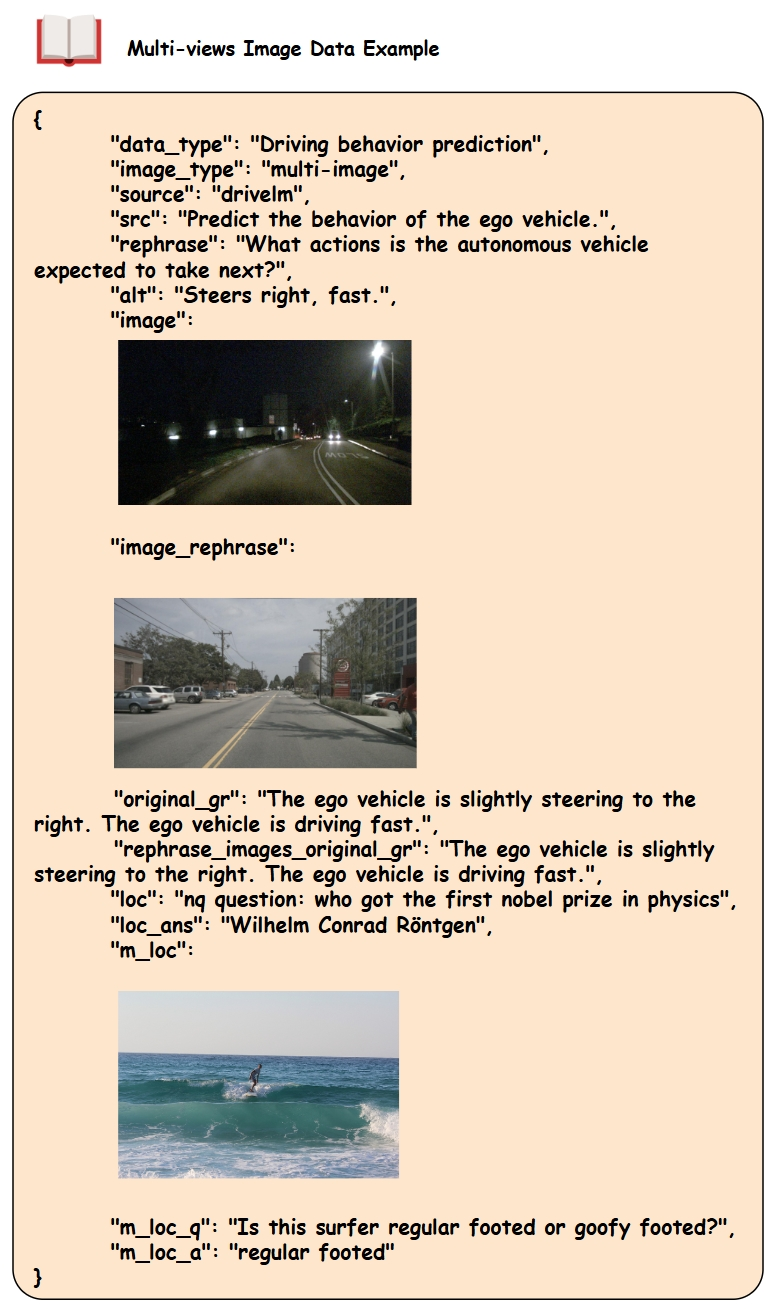}
\caption{A multi-views image data case of \ds benchmark.}
\label{fig:multi_case} 
\end{figure*}

\begin{figure*}[ht] 
\centering
\includegraphics[width=0.6\textwidth]{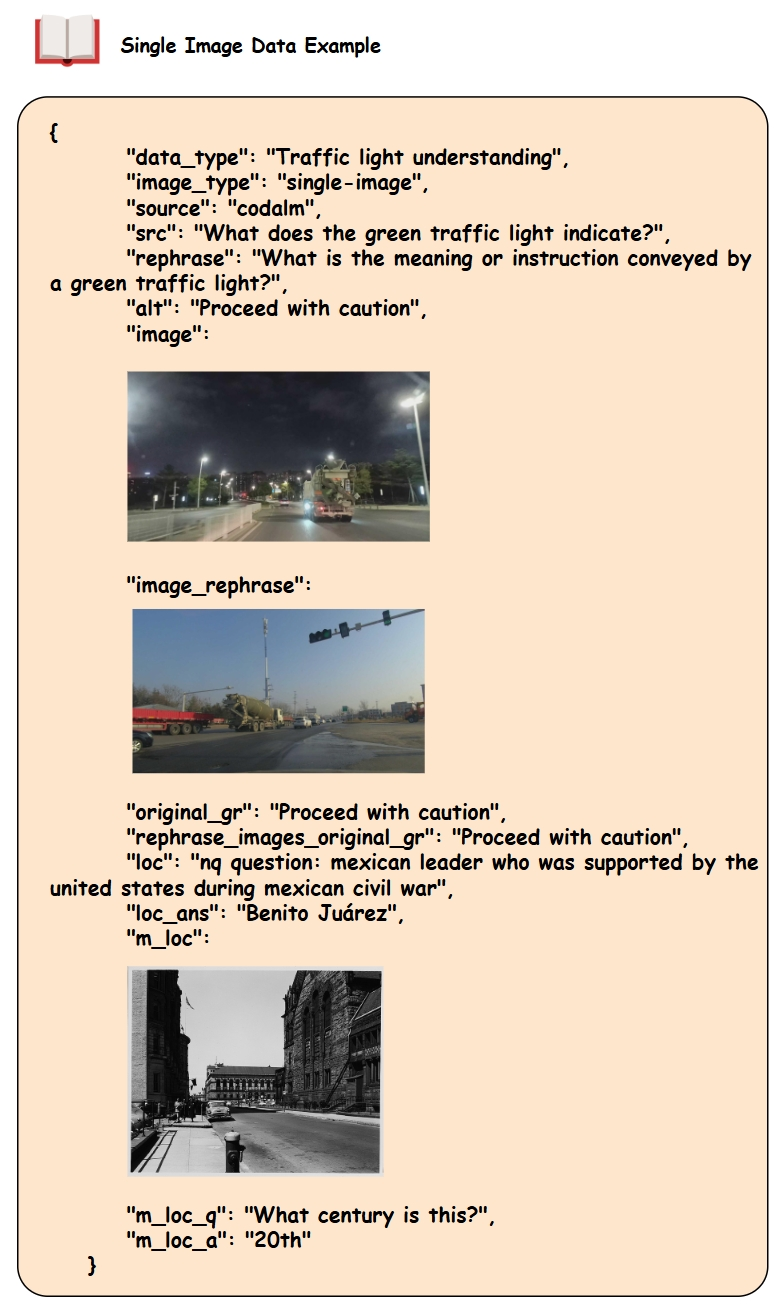}
\caption{A single image data case of \ds benchmark.}
\label{fig:single_case} 
\end{figure*}
